# Supplementary material for: Localized Faraday patterns under heterogeneous parametric excitation
Source: arXiv:1702.02683 source file (2019-03-14)
Supplement: Supplementary file 1 [file SupplementalMaterial_final.pdf]

# Supplemental Material:

## Localized Faraday patterns with inhomogeneous parametric excitation

Héctor Urrea, Saliya Coulibaly, Leonardo Gordillo, and Mónica A. García-Ñustes

### SOLUTIONS OF LINEARIZED PDNLS EQUATION WITH AN INHOMOGENEOUS FORCING $\gamma(x)$

The prototype model describing the dynamics of unidimensionally extended systems in the vicinity of Faraday instability regime is the parametrically driven and damped nonlinear Schrodinger equation,

$$\partial_t A = -i\nu A - i|A|^2 A - i\partial_{xx} A - \mu A + \gamma \bar{A}. \quad (1)$$

To analyze the effect of inhomogeneous forcing, we promote the forcing  $\gamma$  to be a function describing the spatial profile of the forcing, i.e.  $\gamma \equiv \gamma(x)$ . After linearizing Eq. (1) around the trivial homogeneous steady state, we get the a set of equations, one for  $A$ , and another for  $\bar{A}$ :

$$[\partial_t + i\nu + i\partial_{xx} + \mu] A = \gamma(x) \bar{A}, \quad (2)$$

$$[\partial_t - i\nu - i\partial_{xx} + \mu] \bar{A} = \gamma(x) A. \quad (3)$$

We define the linear operators  $\mathcal{L} \equiv \partial_t + i\nu + i\partial_{xx} - \mu$ , and  $\bar{\mathcal{L}}$ , its conjugate operator. After applying  $\bar{\mathcal{L}}$  to (2), and replacing  $\bar{\mathcal{L}}\bar{A}$  by  $\gamma(x) A$  using (3), we can write,

$$\left[ (\partial_t + \mu)^2 + (\nu + \partial_{xx})^2 \right] A - \gamma^2(x) A = 0. \quad (4)$$

Here we have assumed that  $\gamma(x)$  is a slowly varying function of the space ( $\partial_{xx}\gamma \ll 1$ ).

For the sake of simplicity, we now assume that the profile of the energy is of Gaussian type:

$$\gamma(x) = \gamma_i e^{-x^2/2\sigma_i^2}, \quad (5)$$

where  $\gamma_i$  is the amplitude of the forcing and  $\sigma_i$  is the Gaussian standard deviation. In general,  $\gamma_i$  can be any localized function satisfying the three following features: i)  $\gamma(x)$  is symmetric with respect to some  $x_0$ , ii)  $\gamma(x)$  has a single extremum at  $x_0$ , with a non-vanishing second derivative, and iii) decays to 0 as  $x \rightarrow \pm\infty$ .

The degree of inhomogeneity of the system can be modeled through the parameter  $\varepsilon \equiv 1/\sigma_i$ . Introducing the slowly varying variable  $X \equiv \varepsilon x$ , Eq.(5) becomes:

$$\left[ (\partial_t + \mu)^2 + (\nu + \varepsilon^2 \partial_{XX})^2 \right] A - \gamma^2(X) A = 0. \quad (6)$$

A particularly well-suited approach to find solutions in the limit  $\varepsilon \ll 1$  is the WKBJ approximation [1]. We recall that  $\varepsilon \ll 1$  is equivalent to having a small pattern wavelength compared to the characteristic distance of amplitude variations. Thus, we propose the following expansion,

$$A(X, t) = [A_0(X) + \varepsilon A_1(X) + \mathcal{O}(\varepsilon^2)] e^{-i\omega t} e^{\left[ \frac{i}{\varepsilon} \int_{X_s}^X k(X) dX \right]}, \quad (7)$$

where  $A(X \rightarrow \infty, t, \varepsilon) = 0$ ,  $k(X)$  is the pattern wavenumber, and  $X_s$  is the *source* point where the inhomogeneous profile is centered. Substituting the expansion (7) in (6), we obtain at zeroth-order ( $\varepsilon^0$ ), the dispersion relation

$$(-i\omega + \mu)^2 + (\nu - k^2)^2 - \gamma^2(X) = 0 \quad (8)$$

where  $\omega \equiv \omega(X, k) = -i\mu + i\sqrt{\gamma^2(X) - (\nu - k^2)^2}$ .

At the next order  $\mathcal{O}(\varepsilon)$ , we obtain the equation,  $2k(\nu - k^2) \partial_X A_0 - A_0(\nu - 3k^2) \partial_X k = 0$ . Using relation (8), we can now deduce an expression for  $A_0$ , i.e.

$$A_0 \propto \exp \left[ \frac{-i \int F(k, \omega, \mu, \gamma_0, \nu, X) dX}{\partial \omega / \partial k} \right], \quad (9)$$

where  $F(k, \omega, \mu, \gamma_0, \nu, X) \equiv \frac{\nu - 3k^2}{-i\omega + \mu} \partial_X k$ . It is clear that for  $\partial\omega/\partial k = 0$ , expression (9) is singular. The points where the singularity  $\partial\omega/\partial k = 0$  take place are called turning points [1]. On these points, the WKB approach is not longer valid. Let be  $\omega_0 \equiv \omega(k_0)$ , where  $k_0$  is such that

$$\left. \frac{\partial\omega(X)}{\partial k} \right|_{k=k_0} = 0. \quad (10)$$

By definition, if the contour in the complex plane  $\text{Im}[\omega_0(X)]$  exhibits a contact line or pinch between two branches  $X^\pm(\omega_0)$  in a turning point  $X^t$  that also verifies  $\partial\omega_0(X^t)/\partial_X = 0$ , then we deal with a double turning point [2–6]. In that case, the scaling law that rules the system dynamics in the region close to the double turning point is  $X = \varepsilon^{1/2}y$ . In consequence, the expansion takes the following new form,

$$A(y, t) = [A_0(y) + \varepsilon^{1/2}A_1(y) + \mathcal{O}(\varepsilon)]e^{-i\omega t}e^{\left[\frac{i}{\varepsilon^{1/2}}\int_{y_s}^y k(y) dy\right]}. \quad (11)$$

As in the homogeneous case, we have two solutions for  $\partial\omega/\partial k = 0$ , i)  $k_c = 0$  and ii)  $k_c = \pm\sqrt{\nu}$  with  $\nu > 0$ , which correspond respectively to the angular frequencies

$$\omega(k_c) = i\left(-\mu + \sqrt{\gamma^2(X) - \nu^2}\right) \quad \text{and} \quad (12)$$

$$\omega(k_c) = i(-\mu + \gamma(X)). \quad (13)$$

Imposing the second condition ( $\partial\omega/\partial X = 0$ ) for the double turning point, it follows that  $X^t = 0$  for both cases. On the contrary, for different  $k_c$ , we have different values of  $\gamma^t$ . For Faraday waves ( $\nu > 0$ ,  $\gamma > \mu$ ), the critical wavelength is  $k_c = \pm\sqrt{\nu}$  and  $\gamma^t = \mu$ .

After making the corresponding replacements in the parameter expansions and provided that  $\varepsilon \ll 1$ , the spatial forcing takes the form  $\gamma(x) = \gamma_i(1 - \varepsilon(y - y^t)^2/2 + \mathcal{O}(\varepsilon^2))$ . We hence introduce small deviations from the turning point  $\{X^t, \gamma^t\}$  through

$$\gamma = \gamma^t + \varepsilon\gamma^{(1)} + \mathcal{O}(\varepsilon^2), \quad (14)$$

$$\omega = \omega^t + \varepsilon\omega^{(1)} + \mathcal{O}(\varepsilon^2). \quad (15)$$

Thus, we get the expression for the forcing in the turning point,  $\gamma(y) = \gamma^t + \varepsilon[\gamma^{(1)} - \gamma_0^t(y - y^t)^2/2] + \mathcal{O}(\varepsilon^2)$ . At dominant order,  $k = k_c = \sqrt{\nu}$  and Eq. (11) reduces to  $A(y, t) \sim \exp[i\int \sqrt{\nu} dy/\varepsilon^{1/2}]$  [4]. Next, we replace  $A(y, t)$  in (2) and (3) and analyze the equations order by order in  $\varepsilon$ . At order  $\mathcal{O}(\varepsilon^0)$ , we obtain that  $A_0 = \bar{A}_0$ . At order  $\mathcal{O}(\varepsilon^{1/2})$ , we get the relation

$$\mu(A_1 - \bar{A}_1) = 2\sqrt{\nu}\partial_y A_0. \quad (16)$$

Finally at order  $\mathcal{O}(\varepsilon)$ , using  $A_0 = \bar{A}_0$  and relation Eq. (16), we obtain a *Weber equation* that describes the linear behavior of the signal envelope  $A_0$ ,

$$\partial_y^2 A_0 + (\beta^2 - \alpha y^2) A_0 = 0 \quad (17)$$

where  $\alpha \equiv \mu^2/4\nu$  and  $\beta^2 \equiv \mu(\gamma^{(1)}/2\nu + i\omega^{(1)}/2\nu)$ . The solutions of (17) are Hermite polynomials with a Gaussian modulation, i.e.  $A_0 = H_m(\alpha^{1/4}y)e^{-(\sqrt{\alpha}/2)y^2}$ . Due to the discrete spectrum of the linear operator in (17), we also require  $\beta^2/\sqrt{\alpha} = 2m + 1$ , which imposes conditions over  $\gamma^{(1)}$  and  $\omega^{(1)}$ . In terms of the original variable  $x$ , the solution is,

$$A_0(x) = H_\nu\left(\alpha^{1/4}\sigma_i^{-1/2}x\right)e^{-x^2/2\sigma_w^2}$$

where  $H_m$  are the Hermite polynomials and the standard deviation  $\sigma_w$  is given as

$$\sigma_w^2 \equiv \left(\frac{1}{\sqrt{\alpha}}\right)\sigma_i = \left(\frac{2\sqrt{\nu}}{\mu}\right)\sigma_i.$$

We have shown that a weak spatial dependence of  $\gamma$  generates a modulation on the wave pattern given by an amplitude equation equivalent to a Weber-equation eigenvalue problem.

- 
- [1] C. M. Bender and S. A. Orszag, *Advanced mathematical methods for scientists and engineers*, edited by E. H. Spanier and G. Springer, International series in pure and applied mathematics (McGRAW-HILL, 1978).
  - [2] P. Huerre, *Annu. Rev. Fluid Mech.* **22**, 473 (1990).
  - [3] P. A. Monkewits, P. Huerre, and J.-M. Chomaz, *J. Fluid Mech.* **251**, 1 (1993).
  - [4] G. Dewel and P. Borckmans, *Phys. Lett. A* **138**, 189 (1989).
  - [5] M. N. Ouarzazi, P. A. Bois, and M. Taki, *Phys. Rev. A* **53**, 4408 (1996).
  - [6] S. Coulibaly, *Soliton Dissipatifs des oscillateurs Paramétriques optiques: Instabilités convectives/absolues et effets non-linéaires de walk-off*, Ph.D. thesis, Université de Lille I (2006).
